# Supplementary material for: Six loop analytical calculation of the field anomalous dimension and the critical exponent $\eta$ in $O(n)$-symmetric $\varphi^4$ model
Source: arXiv:1601.01960 ancillary file (2016-03-15)
Supplement: Supplementary file 1 [file graphs.pdf]

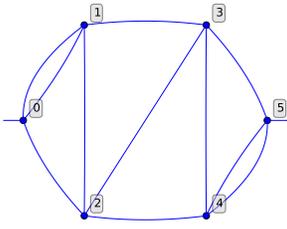

(1)  $e_{112|23|34|45|55|e|}$

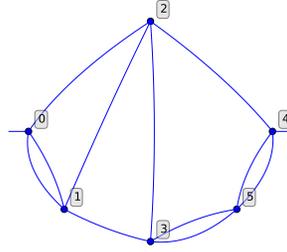

(2)  $e_{112|23|34|55|e55||}$

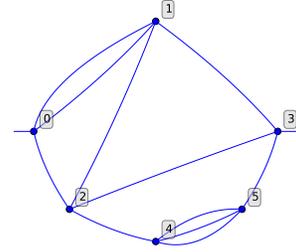

(3)  $e_{112|23|34|e5|555||}$

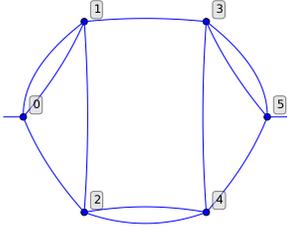

(4)  $e_{112|23|44|455|5|e|}$

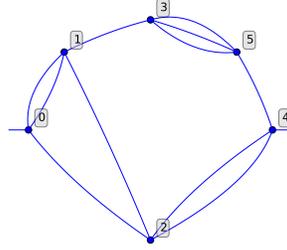

(5)  $e_{112|23|44|555|e5||}$

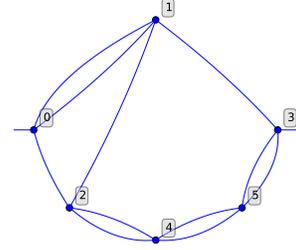

(6)  $e_{112|23|44|e55|55||}$

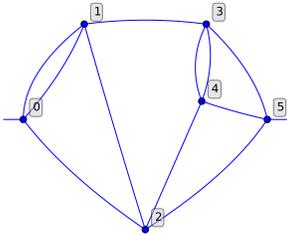

(7)  $e_{112|23|45|445|5|e|}$

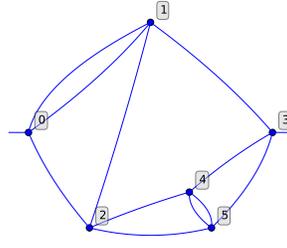

(8)  $e_{112|23|45|e45|55||}$

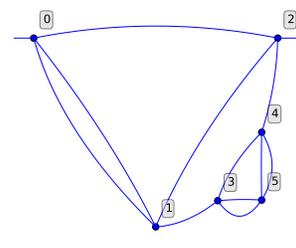

(9)  $e_{112|23|e4|455|55||}$

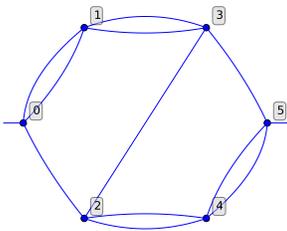

(10)  $e_{112|33|344|5|55|e|}$

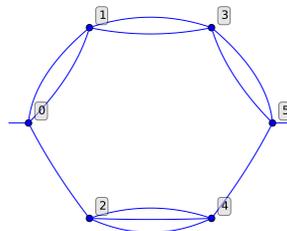

(11)  $e_{112|33|444|55|5|e|}$

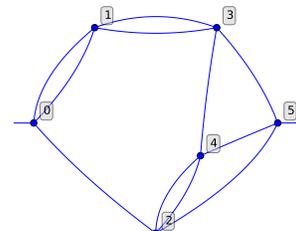

(12)  $e_{112|33|445|45|5|e|}$

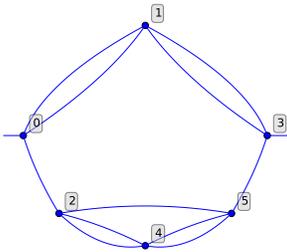

(13)  $e_{112|33|445|e5|55||}$

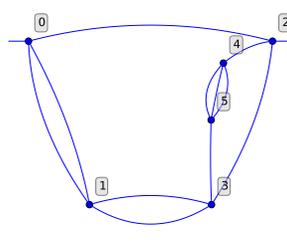

(14)  $e_{112|33|e34|5|555||}$

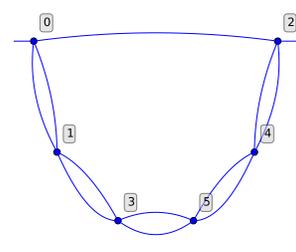

(15)  $e_{112|33|e44|55|55||}$

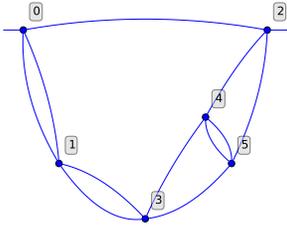

(16)  $e112|33|e45|45|55||$

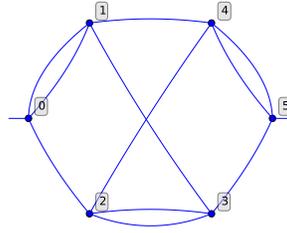

(17)  $e112|34|334|5|55|e|$

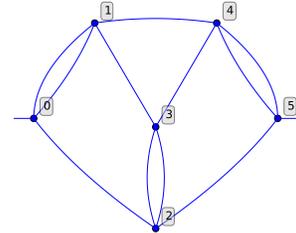

(18)  $e112|34|335|4|55|e|$

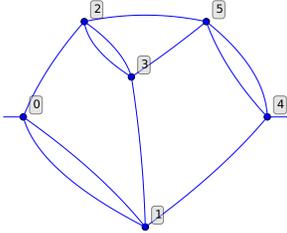

(19)  $e112|34|335|5|e55||$

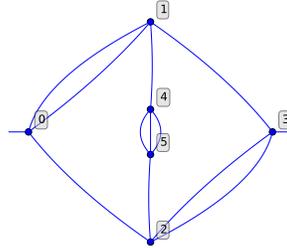

(20)  $e112|34|335|e|555||$

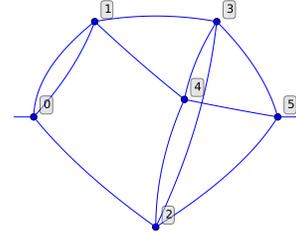

(21)  $e112|34|345|45|5|e|$

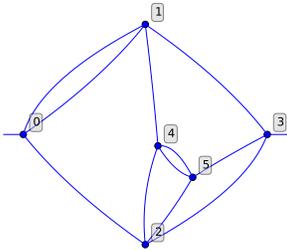

(22)  $e112|34|345|e5|55||$

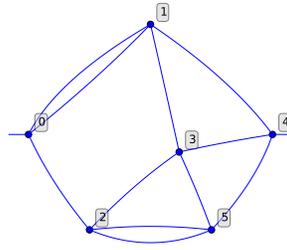

(23)  $e112|34|355|45|e5||$

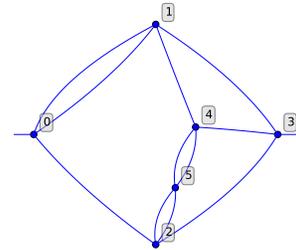

(24)  $e112|34|355|e4|55||$

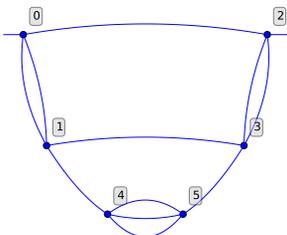

(25)  $e112|34|e33|5|555||$

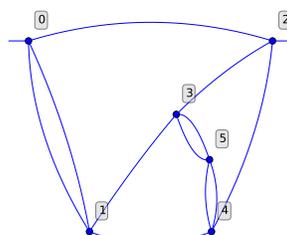

(26)  $e112|34|e34|55|55||$

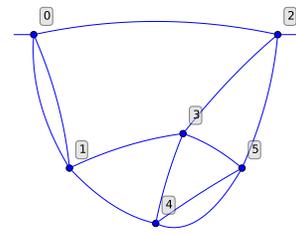

(27)  $e112|34|e35|45|55||$

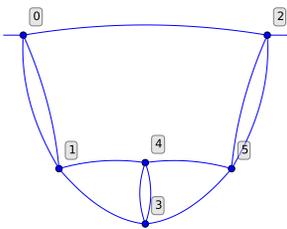

(28)  $e112|34|e55|445|5|5||$

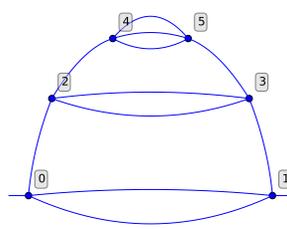

(29)  $e112|e3|334|5|555||$

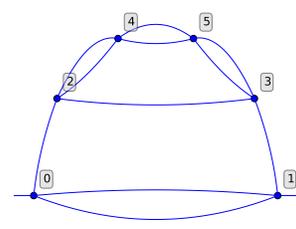

(30)  $e112|e3|344|55|55||$

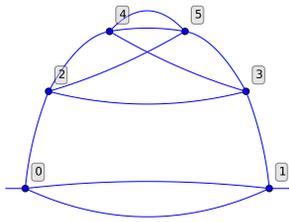

(31)  $e112|e3|345|45|55||$

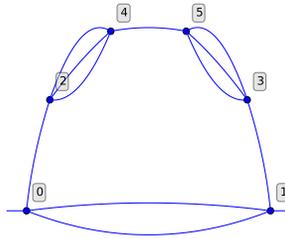

(32)  $e112|e3|444|555|5||$

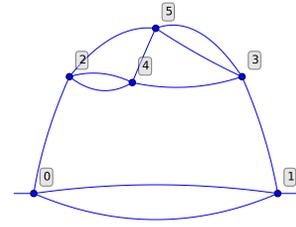

(33)  $e112|e3|445|455|5||$

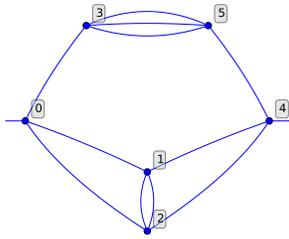

(34)  $e123|224|4|555|e5||$

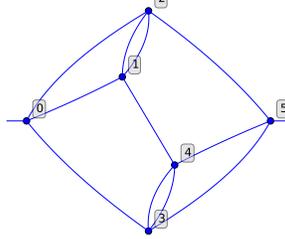

(35)  $e123|224|5|445|5|e||$

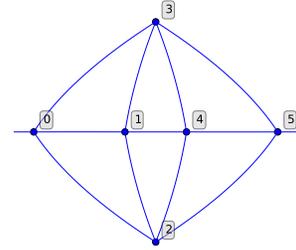

(36)  $e123|234|45|45|5|e||$

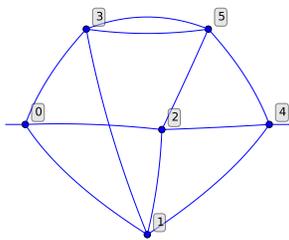

(37)  $e123|234|45|55|e5||$

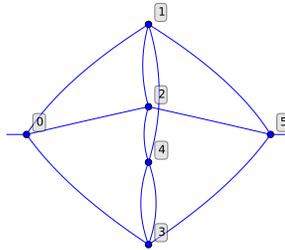

(38)  $e123|245|45|445|e||$

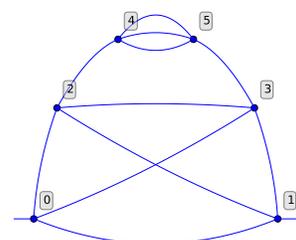

(39)  $e123|e23|34|5|555||$

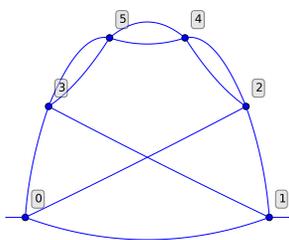

(40)  $e123|e23|44|55|55||$

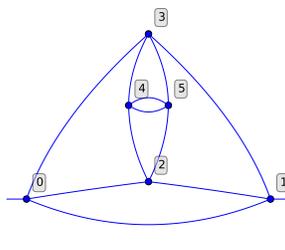

(41)  $e123|e23|45|45|55||$

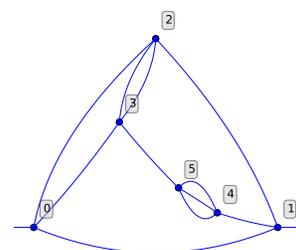

(42)  $e123|e24|33|5|555||$

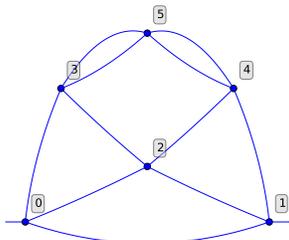

(43)  $e123|e24|34|55|55||$

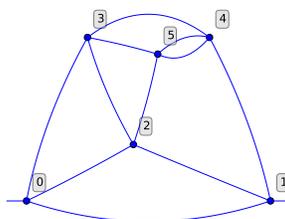

(44)  $e123|e24|35|45|55||$

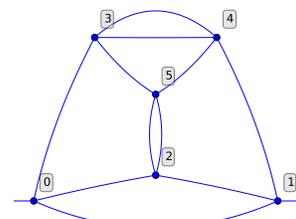

(45)  $e123|e24|55|445|5||$

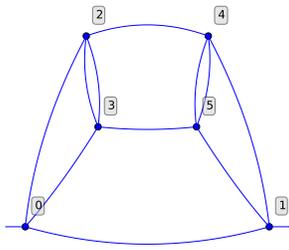

(46)  $e123|e45|334|5|55||$

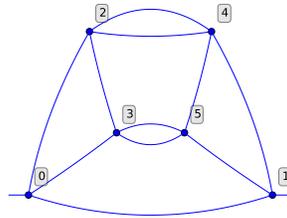

(47)  $e123|e45|344|55|5||$

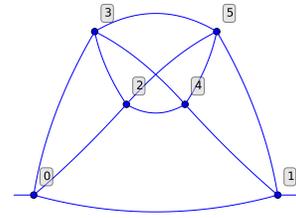

(48)  $e123|e45|345|45|5||$

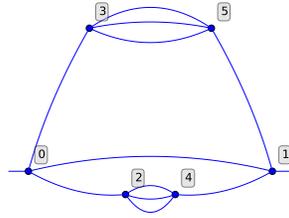

(49)  $e123|e45|444|555|||$

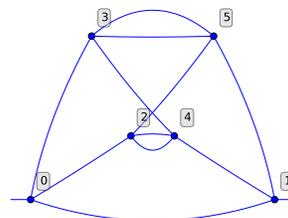

(50)  $e123|e45|445|455|||$
